# Supplementary material for: Is "My Favorite New Movie" My Favorite Movie? Probing the Understanding of Recursive Noun Phrases
Source: arXiv:2112.08326 source file (2022-05-08)
Supplement: Supplementary file 1 [file Annotation_guidlines.pdf]

# NP Data Creation Guide

The goal of our project is to evaluate whether state-of-the-art language models can understand Complex Noun Phrases (NPs). For example, if someone is "*a **skillful American** violinist*" and "*a father*" at the same time, then he is "*an American father*" but not necessarily "*a skillful father*". We would like you to help **create examples of this style** to expand our dataset!

In essence, you need to fill out a spreadsheet like this:

| NP                              | Modified NP                   | TE_prefix | modx+n2_test                             | modx+n2_control                            | event_more_likely                 | event_equally_likely | event_less_likely            | Penn1D       | note |
|---------------------------------|-------------------------------|-----------|------------------------------------------|--------------------------------------------|-----------------------------------|----------------------|------------------------------|--------------|------|
| the skillful American violinist | a skillful American violinist | He is     | a skillful [father]; a skillful [driver] | an American [father]; an American [driver] | plays in a professional orchestra | has a violin         | Berlin is the hometown of [] | xxxxxx<br>xx |      |

You'll be provided with the first column, and fill in the rest. This guide will walk you through what each column means.

|                                         |    |
|-----------------------------------------|----|
| Estimated Time                          | 2  |
| List of terms                           | 3  |
| How annotation works                    | 4  |
| Multi-Premise Textual Entailment (MPTE) | 4  |
| Event Plausibility Change (EPC)         | 5  |
| Annotation Format                       | 6  |
| More examples                           | 11 |
| Tips                                    | 11 |
| Common mistakes                         | 11 |
| How scoring works                       | 13 |
| Getting Started                         | 14 |
| Questions?                              | 14 |

---

## Estimated Time

This is a rather complex task, which will take **30min-45min** to learn.

After that, it will take **30min - 1h** to complete each set of annotations (5 NPs), depending on your proficiency. That's worth **25 points** at maximum.

You can earn up to **100** points in this assignment, equivalent to **1%** of your final grade in the course. That's gonna take **2.5-4.75h** in total (30-45min learning + 2h-4h annotation). You don't have to do it all at once. For more details, see "[How scoring works](#)".

## List of terms

We'll use the following terms throughout the document. You can **take a quick look and go back anytime**.

| Term | Explanation                                                     | Example                                                                                                                                                                                        |
|------|-----------------------------------------------------------------|------------------------------------------------------------------------------------------------------------------------------------------------------------------------------------------------|
| DET  | Determiner                                                      | "a", "the"                                                                                                                                                                                     |
| M    | Modifier                                                        | "skillful", "American", "second"                                                                                                                                                               |
| N    | Noun                                                            | "violinist", "father"                                                                                                                                                                          |
| NP   | Noun Phrase<br>(typically in the form of "DET M1 M2 N")         | "a skillful American violinist"                                                                                                                                                                |
| TE   | Textual Entailment<br>(a task format)                           | <i>A premise <b>entails</b> a hypothesis</i> iff:<br>whenever the premise is true, the hypothesis must be true.<br>e.g. "He can run fast" <b>entails</b> "He can run"<br>(but not vice versa). |
| P    | Prefix in TE                                                    | A prefix in TE premise/hypothesis, e.g.<br>"This is/He is/She is" ...<br>See more details under "How annotation works"!                                                                        |
| MPTE | Multi-Premise Textual Entailment<br>(TE with $\geq 1$ premises) | The <i>premises</i> "He is a boy" and "He is tall" <b>collectively entail</b> the <i>hypothesis</i> "He is a tall boy".<br>See more details under "How annotation works"!                      |
| EPC  | Event Plausibility Change<br>(a task format)                    | The event "A false key can open the door" is less likely than "A key can open the door".<br>See more details under "How annotation works"!                                                     |

# How annotation works

Given an NP, your task is to **write examples** for two tasks we define: **Multi-Premise Textual Entailment** and **Event Plausibility Change**.

## Multi-Premise Textual Entailment (MPTE)

This is the first task.

### Definition

Given two premises and a hypothesis, the task is to decide whether the two premises **collectively entail** the hypothesis.

### Examples

Premise 1: He is a skillful American violinist.

Premise 2: He is a father.

Hypothesis: He is a skillful father.

Label: Non-entailment

Premise 1: He is a skillful American violinist.

Premise 2: He is a father.

Hypothesis: He is an American father.

Label: Entailment

### What you'll need to do

You will be **provided with the NP in Premise 1**, and your task is to:

- a. **come up with an appropriate new noun** (that can **refer to the same entity**) in Premise 2, and
- b. **create the hypothesis**.

More detailed instructions below.

### Intuition

This task tests if a modifier in an NP can be *freely composed with another noun*. For example, “skillful” can’t, but “American” can.

## Formalization

An MPTE example has two premises, a hypothesis, and a label.

Denote the given NP by  $DET\ M_1\ M_2\ N$ . An MPTE example has the following pattern:

Premise 1:  $P\ DET\ M_1\ M_2\ N$ .

Premise 2:  $P\ DET\ N_2$ .

Hypothesis:  $P\ DET\ (M_1\ or\ M_2)\ N_2$ .

Label: Entailment / Non-entailment

Explanation:

1. Both premises start with a **prefix P** (e.g. "This is", "He is", "She is", "Those are"..., depending on the NP).
2. Premise 1 contains the original NP.
3. Premise 2 contains a new noun  $N_2$ , which is different from  $N$ . But it should **refer to the same entity** as  $N$ .
4. Hypothesis contains the **composition of one of the modifiers** and the new noun.
5. The label means whether the two premises together entail the hypothesis.

Example:

$P = \text{He is, } DET\ M_1\ M_2\ N = \text{a skillful American violinist, } N_2 = \text{father}$

Premise 1: He is a skillful American violinist.

Premise 2: He is a father.

Hypothesis: He is a skillful father.

Label: Non-entailment

## Event Plausibility Change (EPC)

This is the second task.

### Definition

Given two events, the task is to decide whether Event 2 is more/equally/less likely to happen than Event 1.

### Examples

Event 1: A child can ride a lion.

Event 2: A child can ride a white stone lion.

Label: More likely

Event 1: A lion is big.

Event 2: A white stone lion is big.

Label: Equally likely

Event 1: A lion can roar.

Event 2: A white stone lion can roar.

Label: Less likely

## What you'll need to do

You will be provided with **the full NP (DET M1 M2 N)**, and your task is to come up with **appropriate events** that are more/equally/less plausible for **the full NP** than **the bare DET N**. More detailed instructions below.

## Intuition

This task tests **how different attributes of a noun will be influenced** once we add modifiers to it.

## Formalization

An EPC example has two events (with the same “event content”  $E$ ) and a label.

Denote the given NP by  $DET\ M_1\ M_2\ N$ . An EPC example has the following pattern:

Event 1:  $Det\ N\ E$ .

Event 2:  $Det\ M_1\ M_2\ N\ E$ .

Label: More/Equally/Less likely

Explanation:

1. The two events have the same “event content”  $E$ . In other words, they only differ in that Event 1 contains the unmodified NP, and Event 2 contains the given NP.
2. The label means whether Event 2 is more/equally/less likely to happen than Event 1.

Example:

$E = \text{can roar,}$       $DET\ M_1\ M_2\ N = \text{a white stone lion}$

Event 1: A lion can roar.

Event 2: A white stone lion can roar.

Label: Less likely

## Annotation Format

You will work with .csv files. Each file contains 5 NPs, one in each row. Your job is to create MPTE (Multi-Premise Textual Entailment) and EPC (Event Plausibility Change) examples for each NP by filling in the columns.

A typical row looks like this:

| NP                              | Modified NP                   | TE_prefix | modx+n2_test                             | modx+n2_control                            | event_more_likely                 | event_equally_likely | event_less_likely            | Penn1D   | note |
|---------------------------------|-------------------------------|-----------|------------------------------------------|--------------------------------------------|-----------------------------------|----------------------|------------------------------|----------|------|
| the skillful American violinist | a skillful American violinist | He is     | a skillful [father]; a skillful [driver] | an American [father]; an American [driver] | plays in a professional orchestra | has a violin         | Berlin is the hometown of [] | 12345678 |      |

Check out more samples [here!](#)

There are 10 columns in each row. The first is given, and you need to fill in **the other 9** if possible. We'll illustrate their meaning using the sample row above:

| NP                              | Modified NP | TE_prefix | modx+n2_test | modx+n2_control | event_more_likely | event_equally_likely | event_less_likely | Penn1D | note |
|---------------------------------|-------------|-----------|--------------|-----------------|-------------------|----------------------|-------------------|--------|------|
| the skillful American violinist |             |           |              |                 |                   |                      |                   |        |      |

1. **NP**: The given NP. You should not change this column.

| NP                              | Modified NP                   | TE_prefix | modx+n2_test | modx+n2_control | event_more_likely | event_equally_likely | event_less_likely | Penn1D | note |
|---------------------------------|-------------------------------|-----------|--------------|-----------------|-------------------|----------------------|-------------------|--------|------|
| the skillful American violinist | a skillful American violinist |           |              |                 |                   |                      |                   |        |      |

2. **Modified NP** (optional): If you need to, you can **modify the NP** (i.e. edit it slightly) as explained below:

You can modify it **whenever it makes it easier** for you to write MPTE and EPC examples. For instance:

- a. There's a **proper name** in the NP.  
e.g. "Abiola's presumed electoral victory", which can be modified to "her presumed electoral victory"
- b. There is a **definite determiner** in the NP.  
e.g. "the mythical wild beast". \*\*\*It's generally recommended to **change it to an indefinite determiner ("a"/"an")** whenever possible\*\*\*, since "the" might bring complications for entailment judgments.
- c. The NP is **plural**, but you think it's more convenient to use the single form.  
e.g. "Several previous official deadlines" -> "its previous official deadline".

- d. In summary, the rule of thumb: Your goal is to make the NP fit perfectly into the MPTE and EPC examples!

The **rest columns will be based on** your modified NP.

| NP                              | Modified NP                   | TE_prefix | modx+n2_test | modx+n2_control | event_more_likely | event_equally_likely | event_less_likely | Penn1D | note |
|---------------------------------|-------------------------------|-----------|--------------|-----------------|-------------------|----------------------|-------------------|--------|------|
| the skillful American violinist | a skillful American violinist | He is     |              |                 |                   |                      |                   |        |      |

3. **TE\_prefix**: The [prefix P](#) for MPTE (Multi-Premise Textual Entailment). The default is "This is". If you feel that this is good enough, leave the column **blank**. Otherwise, choose **one** of "He is"/"She is"/"They are"/"Those are"/"These are". Sometimes you can also use "has/have" (e.g. when the NP is "clear blue eyes"), but **only if necessary** (See more details under [Common Mistakes no. 5](#)).

| NP                              | Modified NP                   | TE_prefix | modx+n2_test                             | modx+n2_control | event_more_likely | event_equally_likely | event_less_likely | Penn1D | note |
|---------------------------------|-------------------------------|-----------|------------------------------------------|-----------------|-------------------|----------------------|-------------------|--------|------|
| the skillful American violinist | a skillful American violinist | He is     | a skillful [father]; a skillful [driver] |                 |                   |                      |                   |        |      |

4. **Modx+n2\_test**: The [DET](#) ( $M_1 | M_2$ )  $N_2$  part in the [MPTE \(Multi-Premise Textual Entailment\) hypothesis](#), such that the label is **Non-Entailment**. (This is a *test* example because it's the minority case.) For instance, "a skillful [father]" in our sample row means that we can form the following MPTE example

Premise 1: He is a skillful American violinist.

Premise 2: He is a father.

Hypothesis: He is a skillful father.

Label: Non-entailment

Note:

- Please **put  $N_2$  (the new noun) in square brackets**, i.e. "[ ]".
- \*\*\* Please make sure that  $N_2$  **can indeed refer to the same entity** as the original NP, i.e. the **two premises can hold** at the same time. \*\*\*  
For instance, "rabbit" would be a bad  $N_2$ , since a violinist is unlikely a rabbit XD.
- If you can think of multiple such phrases, separate them with a ";" (no space in between), e.g. "a skillful [father]; a skillful [driver]".
- Please **write all phrases in full**; don't omit the determiner, and don't condense them with things like "/" or "&".

| NP                              | Modified NP                   | TE_prefix | modx+n2_test                             | modx+n2_control                            | event_more_likely | event_equally_likely | event_less_likely | Penn1D | note |
|---------------------------------|-------------------------------|-----------|------------------------------------------|--------------------------------------------|-------------------|----------------------|-------------------|--------|------|
| the skillful American violinist | a skillful American violinist | He is     | a skillful [father]; a skillful [driver] | an American [father]; an American [driver] |                   |                      |                   |        |      |

5. **Modx+n2\_control**: The **DET** ( $M_1 | M_2$ )  $N_2$  part in the [MPTE hypothesis](#), such that the label is **Entailment**. (This is a *control* example because it's the majority case.) For instance, "an American [father]" in our sample row means that we can form the following MPTE example

Premise 1: He is a skillful American violinist.

Premise 2: He is a father.

Hypothesis: He is an American father.

Label: Entailment

Note:

Same as above. And,

- The control example and the test example can have the same or different  $N_2$ .
- The control example and the test example can have the same or different  $M$ .
- It's **not** the case that the test example has to use  $M_1$  (the first modifier) and the control example has to use  $M_2$  (the second), as in the current example.

Instead, we can have cases like:

NP: "counterfeit foreign cigarettes"

modx+n2\_test: "foreign [products]" (which uses  $M_2$ )

modx+n2\_control: "counterfeit [products]" (which uses  $M_1$ )

| NP                              | Modified NP                   | TE_prefix | modx+n2_test                             | modx+n2_control                            | event_more_likely                 | event_equally_likely | event_less_likely | PennD | note |
|---------------------------------|-------------------------------|-----------|------------------------------------------|--------------------------------------------|-----------------------------------|----------------------|-------------------|-------|------|
| the skillful American violinist | a skillful American violinist | He is     | a skillful [father]; a skillful [driver] | an American [father]; an American [driver] | plays in a professional orchestra |                      |                   |       |      |

6. **Event\_more\_likely**: The **E** part in an [EPC \(Event Plausibility Change\) example](#), such that the label is **More Likely** (after adding the two modifiers to the noun).

Note:

- If the NP *appears before* the event, then the event should be in normal text form. e.g. "plays in a professional orchestra" in our sample row means that we can form the following EPC example:

Event 1: A violinist plays in a professional orchestra.

Event 2: A skillful American violinist plays in a professional orchestra.

Label: More likely

- If the NP occurs in the middle/after the event, then the event should contain a "[]" where the NP fits in.

e.g. "Berlin is the hometown of []" in our sample row means that we can form the following EPC example:

Event 1: Berlin is the hometown of a violinist.

Event 2: Berlin is the hometown of a skillful American violinist.

Label: Less likely

- Sometimes, it might be hard to directly compare "N" and "M1 M2 N". For instance, it's hard to say which of the following it's more likely:

Event 1: A vase is worth a lot of money.

Event 2: An alleged antique vase is worth a lot of money.

This is because a “common” vase is probably cheap, and an “alleged antique” vase is also probably cheap.

But it’s easy to compare “**M2** N” and “M1 M2 N”:

Event 1: A antique vase is worth a lot of money.

Event 2: An alleged antique vase is worth a lot of money.

Label: Less likely

In that case, you can still write this event, but please **make a note** (in the form of “M2”) in the last column, **Note**.

| NP                              | Modified NP                   | TE_prefix | modx+n2_test                             | modx+n2_control                            | event_more_likely                 | event_equally_likely | event_less_likely | PennID | note |
|---------------------------------|-------------------------------|-----------|------------------------------------------|--------------------------------------------|-----------------------------------|----------------------|-------------------|--------|------|
| the skillful American violinist | a skillful American violinist | He is     | a skillful [father]; a skillful [driver] | an American [father]; an American [driver] | plays in a professional orchestra | has a violin         |                   |        |      |

7. **Event\_equally\_likely**: The **E** part in an **EPC example**, such that the label is **Equally Likely** (after adding the two modifiers to the noun).

Note:

Same as above.

| NP                              | Modified NP                   | TE_prefix | modx+n2_test                             | modx+n2_control                            | event_more_likely                 | event_equally_likely | event_less_likely            | PennID | note |
|---------------------------------|-------------------------------|-----------|------------------------------------------|--------------------------------------------|-----------------------------------|----------------------|------------------------------|--------|------|
| the skillful American violinist | a skillful American violinist | He is     | a skillful [father]; a skillful [driver] | an American [father]; an American [driver] | plays in a professional orchestra | has a violin         | Berlin is the hometown of [] |        |      |

8. **Event\_less\_likely**: The **E** part in an **EPC example**, such that the label is **Less Likely** (after adding the two modifiers to the noun).

Note:

Same as above.

| NP                              | Modified NP                   | TE_prefix | modx+n2_test                             | modx+n2_control                            | event_more_likely                 | event_equally_likely | event_less_likely            | PennID   | note |
|---------------------------------|-------------------------------|-----------|------------------------------------------|--------------------------------------------|-----------------------------------|----------------------|------------------------------|----------|------|
| the skillful American violinist | a skillful American violinist | He is     | a skillful [father]; a skillful [driver] | an American [father]; an American [driver] | plays in a professional orchestra | has a violin         | Berlin is the hometown of [] | 12345678 |      |

9. **PennID**: Your PennID (an 8-digit number; **not** your PennKey!).

You can auto-fill all of those in at once with your favorite editor (e.g. Excel/Numbers)!

| NP                              | Modified NP                   | TE_prefix | modx+n2_test                             | modx+n2_control                            | event_more_likely                 | event_equally_likely | event_less_likely            | PennID   | note |
|---------------------------------|-------------------------------|-----------|------------------------------------------|--------------------------------------------|-----------------------------------|----------------------|------------------------------|----------|------|
| the skillful American violinist | a skillful American violinist | He is     | a skillful [father]; a skillful [driver] | an American [father]; an American [driver] | plays in a professional orchestra | has a violin         | Berlin is the hometown of [] | 12345678 |      |

10. **Note**(optional): If there's anything you're unsure of or needs manual post-editing (e.g. "m2" for the three events), leave a note here.

## More examples

We recommend **taking a look at the [sample spreadsheet](#)** before getting started! You'll get an idea of what kind of examples we are looking for.

Note that they are only a style reference; you **shouldn't write anything too similar** to them in your own submission.

## Tips

Please read this if you want to spend your time the most effectively :)

1. If it's too hard to fill in any cell, \*\*\* **don't spend too much time (>5min) on it!** \*\*\* Leave it blank and move on.  
A lot of cells might be intrinsically impossible to fill in. Don't worry about them. Given a fixed amount of time, it's generally more reasonable to **attempt more files** instead of **trying to fill in every cell in a file**. **Quality** matters more than quantity!
2. If there are **weird NPs** (e.g. jargon, ambiguous words, too specific/general terms ...) so that you can't think of any good example, skip it altogether!
3. Edit the .csv file with Excel/Numbers, and export to .csv again once finished.
4. To get inspiration for events, try to search the head noun on [ConceptNet!](#)

## Common mistakes

- a. Grammatical error: The events can't and the NP doesn't make a sentence. Example errors:

| NP                           | event_more_likely                           |
|------------------------------|---------------------------------------------|
| an initial positive response | be the answer someone was hoping to receive |

Instead, it should be "is the answer someone was hoping to receive".

| NP                        | event_more_likely |
|---------------------------|-------------------|
| dubious strategic motives | that we see       |

What does it mean?

- b. Invalid N<sub>2</sub>: The N<sub>2</sub> you write **can't refer to the same entity** as the original NP. Example errors:

| NP                                | TE prefix | modx+n_test        |
|-----------------------------------|-----------|--------------------|
| a surrogate presidential campaign | He has    | a surrogate [wife] |

Though the TE prefix is "He has", the N<sub>2</sub> "wife" can't refer to the same entity as "campaign". Instead, you should use "has/have" very cautiously (**only if you are sure that N<sub>2</sub> refers to the same entity**), e.g.

| NP                     | TE prefix | modx+n_control       |
|------------------------|-----------|----------------------|
| a beautiful young wife | He has    | a beautiful [spouse] |

would be a good example.

| NP                 | modx+n_test      |
|--------------------|------------------|
| a white stone lion | a white [animal] |

If “X is a white stone lion”, then we can’t say “X is an animal” at the same time.

| NP                         | modx+n_test         |
|----------------------------|---------------------|
| a partial federal shutdown | a partial [success] |

Similarly, “a partial federal shutdown” is unlikely a “success” in the first place.

5. **Modx+n2\_test** and **Modx+n2\_control** is swapped:

Note that **Modx+n2\_test** should be **Non-Entailment**, while **Modx+n2\_control** should be **Entailment**. A example error:

| NP                        | modx+n_test           | modx+n_control        |
|---------------------------|-----------------------|-----------------------|
| presumed negative effects | presumed [influences] | negative [influences] |

Instead, the **Modx+n2\_test** and **Modx+n2\_control** columns should be swapped, since:

Premise 1: It has presumed negative effects.

Premise 2: It has influences.

Hypothesis: It has negative influences.

Label: Non-entailment (**Modx+n2\_test**) (i.e. It’s *presumed* to be negative, but it does not necessarily turn out to be indeed negative.)

Premise 1: It has presumed negative effects.

Premise 2: It has influences.

Hypothesis: It has presumed influences.

Label: Entailment (**Modx+n2\_control**)

6. **event\_more\_likely** and **event\_less\_likely** is swapped:

The direction of the comparison should be: whether **DET M1 M2 N** is more/equally/less likely than **DET N**. A example error:

| NP                         | event_more_likely | event_less_likely    |
|----------------------------|-------------------|----------------------|
| a onetime musical director | plays in a band   | We have fired the [] |

Instead, the two cells should be swapped.

# How scoring works

Once you submit your annotation, we will review it and assign credit based on the number of **approved “examples”** you contribute. Specifically,

1. The definition of an “example”:  
In the MPTE task, each “N2” counts as an example.  
In the EPC task, each “event” counts as an example.
2. Each **approved example** will be given 1 point.
3. The top **10% earliest** submissions will receive a 20-point bonus.
4. You can earn up to a total of 100 points (equivalent to **1%** of your overall grade) in extra credit for this assignment. That’s roughly 4-5 files.

\*\*\* **To get the most of your examples approved** \*\*\*, what we are looking for includes:

1. **Semantic & grammatical correctness:**  
First, your sentences should make sense : )  
Please pay attention to details like **number**, **case**, **tense**, etc.
2. **Format correctness:**  
Your submission should be valid .csv files.  
Each example should conform to the format described under “How annotation works”.
3. **Diversity:**  
Please **try to write diversified N2 / events!** (A counterexample would be: whenever there’s an NP like “a previous M2 N”, you’d write “is no longer N” as the “less likely event”). Try to make the content and phrasing as dissimilar as possible!
4. **Non-triviality:**  
Please don’t write trivial examples (e.g. for an NP like “a toy electric car”, you write “is a car” as the “less likely event”; or, you only add a “not” into the “more likely event” to create the “less likely event”).  
Instead, try to think of *properties/things that can happen* about a car (e.g. “can seat four people”).
5. **Class balance:**  
Please try to make your examples as evenly distributed among classes as possible. For instance, the 3 classes, “more/equally/less likely”, should have roughly the same number of examples.

# Getting Started

Thank you for reading all the way here! You are now ready to get started!

If you are unsure of anything, you can first check the instructions/[sample spreadsheet](#) above; or ask under our piazza post.

1. Access the first-round sign-up sheet:  
Go to the [First-round Sign-up Sheet](#). Click “Request Edit Access” under “View only” and send it. We’ll approve it ASAP.  
(We’ve turned off public link sharing because there have been malicious edits from anonymous users.)
2. Sign up for the **first** file:  
Each row in the sign-up sheet stands for a .csv file containing 5 NPs under the [source\\_NP folder](#).  
Choose a file whose **status** is “Available” to claim it. (Please don’t claim >1 just yet!)  
Put your Penn ID in **Annotator Penn ID**.  
Change the **status** to “Claimed”.  
Don’t put anything in **Reviewer**!
3. Download the **first** file:  
Go to the [source\\_NP folder](#), download the file you just claimed.
4. Annotate the **first** file:  
Fill in the contents of the file! For more details, see “How annotation works”.
5. Submit the annotated **first** file:  
Submit your file via this Google form: <https://forms.gle/eTk9AdUNiX1CEZjd9>.  
Also, change the **status** to “Submitted” in the signup sheet. **Only after this** will we review your file.  
Please **\*\*\*don’t change the original filenames\*\*\***!
6. Annotating more files (if you wish):
  - a. If you want to annotate more files, indicate so in the Google form.
  - b. After you change the status to “Submitted”, we’ll look at your first-round file.
  - c. **Wait for our reply!** We’ll assign you to a new sign-up sheet via email. **\*\*\*Don’t sign up for >1 files in the first-round sheet!\*\*\***
  - d. You can now sign up for more files in the new sheet! You can submit multiple times, but please **don’t resubmit** the same file(s).
7. Final submission on Gradescope:  
After you’ve **submitted every annotated file** using the Google form, find the assignment titled “Extra Credit: Data creation for complex NPs” on Gradescope and make a submission by answering the questions there. You don’t need to upload anything there; it’s just for the sake of receiving credit.
8. Grading:  
We’ll release the grades based on all your submissions on Gradescope around 2-3 weeks after the due date.

## Questions?

Please ask under our Piazza post (titled “Extra credit opportunity: Data creation for complex NPs”)! We’ll respond ASAP.

Don’t make a new post! We may not have time to monitor the entire Piazza since we aren’t TAs.
