# Supplementary material for: Is "My Favorite New Movie" My Favorite Movie? Probing the Understanding of Recursive Noun Phrases
Source: arXiv:2112.08326 source file (2022-05-08)
Supplement: Supplementary file 2 [file Annotation_guidlines.pdf]

# NP label creation assignment - Instructions

The goal of this assignment is to benchmark human performance on our dataset about understanding complex Noun Phrases (NPs). We'd like you to **answer the questions** in our dataset for us to see how well humans can do our tasks.

## Estimated Time & Scoring

This is a much easier task than our last assignment. It will only take **10-15 min** to learn.

After that, it will take around **20 seconds** to answer each question. Each **correctly answered** question is worth **1 point**. The maximum you can earn is **600 points**, equivalent to **1% of your overall grade** in extra credit in the course.

That's gonna take around **3.5-4h** in total (10-15 min learning + 200min answering). You don't have to do it all at once. Also, if you don't want to spend that much time, **partial credit** is available.

## Getting Started

### 1. Registration:

Go to the Amazon Mechanical Turk Worker Sandbox

(<https://workersandbox.mturk.com/>), sign in with your Amazon account, and register as a worker.

- a. If you don't have an Amazon account, you may need to create one.
- b. Please remember the email address you used to sign in, since we may contact you through that address later.

### 2. Preview the tasks & Qualification test:

There are 3 tasks in our dataset. You can work on any mix of them as you like.

Before starting on **any task** officially, you'll need to take a **qualification test**. You can preview a task, learn how to do it, and qualify for the official task by taking its test:

\* Please provide your **PennID** (8-digit number, **not** your PennKey) at the start of the test.

| Task name | Qualification Test Link |
|-----------|-------------------------|
|-----------|-------------------------|

|                               |                                                                                                                                                                                                         |
|-------------------------------|---------------------------------------------------------------------------------------------------------------------------------------------------------------------------------------------------------|
| Single-Premise Reasoning      | <a href="https://workersandbox.mturk.com/projects/38DARXH Y8YPOS5QTI9P15I757GK082/tasks?ref=w_pl_prvw">https://workersandbox.mturk.com/projects/38DARXH Y8YPOS5QTI9P15I757GK082/tasks?ref=w_pl_prvw</a> |
| Multi-Premise Reasoning       | <a href="https://workersandbox.mturk.com/projects/3D8B00U5 3R3K9XPQ1W7K7G5CAR038U/tasks?ref=w_pl_prvw">https://workersandbox.mturk.com/projects/3D8B00U5 3R3K9XPQ1W7K7G5CAR038U/tasks?ref=w_pl_prvw</a> |
| Event Plausibility Comparison | <a href="https://workersandbox.mturk.com/projects/3XCJG7TD N8ZJCYHRSSYREZCSYCHWC3/tasks?ref=w_pl_prvw">https://workersandbox.mturk.com/projects/3XCJG7TD N8ZJCYHRSSYREZCSYCHWC3/tasks?ref=w_pl_prvw</a> |

Though there might be multiple HITs (=pages) in each link, you only need to complete **one HIT (10 questions)** and click **“Submit” once**.

Note:

- a. A bug in the Event Plausibility Comparison task: Sometimes you are going to see examples without anything highlighted in green; in this case, please interpret ***everything other than the modified NP*** as the event in green.

For example:

**Q4**

**Sentence 1:** "Together with the European Union, the dozen countries are part of the Iran Nuclear Deal."

**Sentence 2:** "Together with the European Union, the initial half dozen countries are part of the Iran Nuclear Deal."

Adding the underlined modifier(s) makes the **event in green** \_\_\_\_ to happen.

☐ more likely  
☐ equally likely  
☐ less likely  
☐ I don't know which option to choose, because:

OPTIONAL: problem with this question

In this case, please consider "Together with the European Union, ... are part of the Iran Nuclear Deal" as the event.

### 3. Wait for the qualification:

After you submit your answers to a qualification test, we'll grade them within 24h and notify you of the results automatically. Please keep an eye on emails from [mturk-noreply@amazon.com](mailto:mturk-noreply@amazon.com) at the **email address you used at sign-in**.

- a. If you pass, you'll receive an email titled "SANDBOX: Qualification Assigned Notification".  
If you can't find the email after 24h, you can also visit the official task link in Step 4 corresponding to the test you took. You'll be able to "Accept & Work" on it if you are qualified.
- b. If you don't pass, you'll receive an email titled "SANDBOX: [Amazon Mechanical Turk] Qualification Denied Notification".  
Unfortunately, you can't retake the test, but you are welcome to try the other 2

tasks.

4. **Work on the official task:**

Depending on which qualification you get, you can now work on the corresponding official task:

| Task name                     | Official Task Link                                                                                                                                                                                    |
|-------------------------------|-------------------------------------------------------------------------------------------------------------------------------------------------------------------------------------------------------|
| Single-Premise Reasoning      | <a href="https://workersandbox.mturk.com/projects/36M7HST2MEL3BVNX48RUYIVDIYN3BX/tasks?ref=w_pl_prvw">https://workersandbox.mturk.com/projects/36M7HST2MEL3BVNX48RUYIVDIYN3BX/tasks?ref=w_pl_prvw</a> |
| Multi-Premise Reasoning       | <a href="https://workersandbox.mturk.com/projects/3Z18Y091VJHXE9LYM6Z7TF71ZC31FN/tasks?ref=w_pl_prvw">https://workersandbox.mturk.com/projects/3Z18Y091VJHXE9LYM6Z7TF71ZC31FN/tasks?ref=w_pl_prvw</a> |
| Event Plausibility Comparison | <a href="https://workersandbox.mturk.com/projects/3X92HJBC47CH0VREBGIMCDG98MXW80/tasks?ref=w_pl_prvw">https://workersandbox.mturk.com/projects/3X92HJBC47CH0VREBGIMCDG98MXW80/tasks?ref=w_pl_prvw</a> |

Unfortunately, we won't be able to give real-time feedback on how many questions you answered correctly. We'll grade everything at the end instead.

5. **Submit on Gradescope:**

After you finish all questions you'd like to answer, go to the "Extra Credit: Label creation for complex NPs" assignment on Gradescope, fill out the form. This will allow us to give you the credit.

## Questions?

Please ask under our Piazza post ("Extra credit opportunity: Label Creation for Complex NPs")! We'll respond ASAP.

Don't make a new post! We are unable to monitor the entire Piazza since we aren't TAs.
